# Supplementary material for: ZipDepth: Bringing Lightweight Zero-Shot Monocular Depth Anywhere, on Any Device
Source: arXiv:2607.08771 source file (2026-07-09)
Supplement: Supplementary file 1 [file arch_detailed.tex]

\begin{table}[h]
\centering
\caption{\textbf{Detailed ZipDepth architecture.} Each row specifies one functional layer or module. $S$: stride; $K$: kernel size; $G$: groups; $r$: dilation rate. Output spatial dimensions assume an input of $H \!\times\! W$.}
\label{tab:arch_detailed}
\resizebox{\columnwidth}{!}{%
\setlength{\tabcolsep}{5pt}
\small
\begin{tabular}{@{}l l c c c c l@{}}
\toprule
\textbf{Stage} & \textbf{Layer / Module} & \textbf{$K$} & \textbf{$S$} & \textbf{Out Ch.} & \textbf{Resolution} & \textbf{Notes} \\
\midrule
\multicolumn{7}{@{}l}{\textit{\textbf{Encoder}}} \\
\midrule
\multirow{2}{*}{Stem}
  & ConvBN             & 3 & 2 & 24   & $H/2$  & Skip $\mathbf{s}_{1/2}$ to decoder \\
  & ConvBN             & 3 & 2 & 48   & $H/4$  & Enters Stage\,1 \\
\midrule
\multirow{1}{*}{Stage\,1}
  & RepVGG $\times 2$  & 3 & 1 & 48   & $H/4$  & \\
\midrule
\multirow{4}{*}{Stage\,2}
  & RepVGG (downsample) & 3 & 2 & 96  & $H/8$  & Stride-2 transition \\
  & RepVGG $\times 2$  & 3 & 1 & 96   & $H/8$  & \\
  & MinimalMultiScale  & 3 & 1 & 96   & $H/8$  & DWConv $r\!=\!1$ + DWConv $r\!=\!2$ \\
  & StripPoolingAttn   & 1 & -- & 96  & $H/8$  & Sigmoid gate, DW $1\!\times\!1$ \\
\midrule
\multirow{4}{*}{Stage\,3}
  & RepVGG (downsample) & 3 & 2 & 192 & $H/16$ & Stride-2 transition \\
  & RepVGG $\times 6$  & 3 & 1 & 192  & $H/16$ & \\
  & ChannelAttention (SE) & -- & -- & 192 & $H/16$ & Reduction $= 8$; hidden $= 24$ \\
  & GlobalContextBlock & 1 & -- & 192  & $H/16$ & Reduction $= 4$; hidden $= 48$ \\
\midrule
\multirow{2}{*}{Stage\,4}
  & RepVGG (downsample) & 3 & 2 & 384 & $H/32$ & Stride-2 transition \\
  & RepVGG $\times 2$  & 3 & 1 & 384  & $H/32$ & \\
\midrule
\multirow{2}{*}{Post-enc.}
  & SPPF               & 5 & 1 & 384  & $H/32$ & Hidden $= 96$; 3$\times$ cascaded MaxPool \\
  & CrossScale          & 1 & -- & 192, 384 & $H/16$, $H/32$ & Grouped $1\!\times\!1$; scale $= 0.3$ \\
\midrule
\multicolumn{7}{@{}l}{\textit{\textbf{Decoder}}} \\
\midrule
\multirow{4}{*}{FPN Fusion}
  & Proj$_4$ (ConvBN)  & 1 & 1 & 288  & $H/32$ & Project Stage\,4 \\
  & Fuse$_3$           & 1 & -- & 192  & $H/16$ & Stage\,3 skip + $\uparrow$Proj$_4$ \\
  & Fuse$_2$           & 1 & -- & 144  & $H/8$  & Stage\,2 skip + $\uparrow$Fuse$_3$ \\
  & Fuse$_1$           & 1 & -- & 96   & $H/4$  & Stage\,1 skip + $\uparrow$Fuse$_2$ \\
\midrule
\multirow{4}{*}{Half-res head}
  & Fuse$_{1/2}$       & 1 & -- & 32   & $H/2$  & $\mathbf{s}_{1/2}$ skip + $\uparrow$Fuse$_1$ \\
  & DepthHead          & 3 & 1 & 1    & $H/2$  & Intermediate depth $\hat{d}_{1/2}$ \\
  & ConvexUp (GPU)     & 3 & -- & 1    & $H$    & $2\!\times$; 9-neighbour softmax \\
  & GatedUp (NPU)      & 5 & -- & 1    & $H$    & $2\!\times$; gate $1{\times}1$,DW$5{\times}5$,$1{\times}1$ \\
\bottomrule
\end{tabular}
}%
\end{table}
