# Supplementary material for: ZipDepth: Bringing Lightweight Zero-Shot Monocular Depth Anywhere, on Any Device
Source: arXiv:2607.08771 source file (2026-07-09)
Supplement: Supplementary file 2 [file dataset_details.tex]

\begin{table}[h]
\centering
\caption{\textbf{Training datasets.} Per-domain image counts and scene categories.}
\label{tab:dataset_details}
\setlength{\tabcolsep}{8pt}
\small
\resizebox{\linewidth}{!}{%
\begin{tabular}{@{}llr@{}}
\toprule
\textbf{Dataset} & \textbf{Domain / Scene Type} & \textbf{Images} \\
\midrule
SA-1B~\cite{kirillov2023segment}& Web-crawled, diverse & 6\,387\,613 \\
Google Landmarks~\cite{weyand2020GLDv2} & Landmarks, architecture & 3\,358\,709 \\
OpenImages~v7~\cite{OpenImages} & Web-crawled, object-centric & 1\,743\,042 \\
Object365~\cite{shao2019objects365} & Object-centric, indoor/outdoor & 1\,693\,306 \\
COCO~\cite{lin2014microsoft} & Indoor/outdoor, multi-category & 532\,855 \\
DrivingStereo~\cite{yang2019drivingstereo} & Driving, stereo-captured & 169\,894 \\
MegaDepth~\cite{Li2018} & SfM reconstructions, tourism & 128\,315 \\
BDD100K~\cite{yu2020bdd100k} & Driving, diverse weather & 100\,000 \\
HoloPix50K~\cite{hua2020holopix50k} & Stereo, user-generated & 49\,124 \\
ADE20K~\cite{zhou2019semantic} & Indoor/outdoor, semantic scenes & 27\,574 \\
HRWSI~\cite{xian2020structure} & Stereo, high-resolution web & 20\,778 \\
Mapillary~\cite{neuhold2017mapillary} & Street-level, global & 20\,000 \\
Gated2Depth~\cite{gated2depth2019} & Night/adverse driving & 14\,277 \\
Trans10K~\cite{xie2020segmenting} & Transparent objects & 10\,428 \\
ACDC~\cite{sakaridis2021acdc} & Adverse conditions driving & 8\,012 \\
Cityscapes~\cite{Cordts2016Cityscapes} & Urban driving & 5\,000 \\
Flickr1024~\cite{wang2019flickr1024} & Stereo, diverse & 1\,024 \\
\midrule
\textbf{Total} & & \textbf{14\,269\,951} \\
\bottomrule
\end{tabular}
}
\end{table}
