# Supplementary material for: ZipDepth: Bringing Lightweight Zero-Shot Monocular Depth Anywhere, on Any Device
Source: arXiv:2607.08771 source file (2026-07-09)
Supplement: Supplementary file 3 [file runtime.tex]

\begin{table}[H]
\centering
\caption{
  Deployment profiling of ZipDepth at $384\!\times\!384$ resolution. Latency is the median over 200 forward passes (20 warm-up). $\ast$~Conv-BN and reparameterizable branch fusion applied via \texttt{fuse\_for\_inference()}.
  $\ddagger$~TensorRT FP16 engine with static shape. $\dagger$~\texttt{torch.compile} with \texttt{mode="max-autotune"}. $\blacktriangle$~ONNX Runtime; best thread count reported.
  $\lozenge$~NPU/mobile path.
  $\clubsuit$~CoreML with Neural Engine.
}
\label{tab:runtime}
\setlength{\tabcolsep}{4pt}
\resizebox{\linewidth}{!}{%
\begin{tabular}{llcrrr}
\toprule
\multirow{2}{*}{\textbf{Device}}
  & \multirow{2}{*}{\textbf{Backend}}
  & \multirow{2}{*}{\textbf{Prec.}}
  & \textbf{Latency}
  & \multirow{2}{*}{\textbf{FPS}}
  & \textbf{Speedup} \\
  & & & \textbf{(ms)} & & \textbf{(vs.\,Eager)} \\
\midrule
\multirow{5}{*}{\shortstack[l]{NVIDIA RTX 3090\\(24\,GB, 350\,W)}}
  & PyTorch Eager           & FP32 &  3.9 &  255 & $1.0\times$ \\
  & PyTorch Fused$^\ast$    & FP32 &  2.5 &  389 & $1.5\times$ \\
  & PyTorch Fused$^\ast$    & FP16 &  3.2 &  307 & $1.2\times$ \\
  & \texttt{torch.compile}$\dagger$  & FP16 &  0.9 & 1117 & $4.4\times$ \\
  & TensorRT$^\ddagger$     & FP16 & \textbf{0.8} & \textbf{1317} & $\mathbf{5.1\times}$ \\
\midrule
\multirow{5}{*}{\shortstack[l]{NVIDIA RTX 3070\\Laptop (140\,W)}}
  & PyTorch Eager           & FP32 &  3.9 &  249 & $1.0\times$ \\
  & PyTorch Fused$^\ast$    & FP32 &  2.7 &  351 & $1.4\times$ \\
  & PyTorch Fused$^\ast$    & FP16 &  2.9 &  341 & $1.4\times$ \\
  & \texttt{torch.compile}$\dagger$  & FP16 &  2.0 &  492 & $2.0\times$ \\
  & TensorRT$^\ddagger$     & FP16 & \textbf{1.3} & \textbf{773} & $\mathbf{3.1\times}$ \\
\midrule
\multirow{4}{*}{\shortstack[l]{NVIDIA Jetson\\Orin NX 16\,GB\\(MAXN, 50\,W)}}
  & PyTorch Eager           & FP32 & 13.9 &   72 & $1.0\times$ \\
  & PyTorch Fused$^\ast$    & FP32 &  8.5 &  118 & $1.6\times$ \\
  & PyTorch Fused$^\ast$    & FP16 &  8.8 &  114 & $1.6\times$ \\
  & TensorRT$^\ddagger$     & FP16 & \textbf{3.2} & \textbf{196} & $\mathbf{4.3\times}$ \\
\midrule
\multirow{4}{*}{\shortstack[l]{NVIDIA Jetson\\Orin NX 16\,GB\\(15\,W)}}
  & PyTorch Eager           & FP32 & 32.0 &   31 & $1.0\times$ \\
  & PyTorch Fused$^\ast$    & FP32 & 29.0 &   34 & $1.4\times$ \\
  & PyTorch Fused$^\ast$    & FP16 & 23.7 &   42 & $1.4\times$ \\
  & TensorRT$^\ddagger$     & FP16 & \textbf{13.1} & \textbf{77} & $\mathbf{2.9\times}$ \\
\midrule
\multirow{3}{*}{\shortstack[l]{AMD EPYC 7443\\(24-core, 200\,W)}}
  & PyTorch Fused (CPU)$^\ast$              & FP32 & 19.8 & 50  & $1.0\times$ \\
  & PyTorch JIT Frozen (CPU)              & FP32 & 18.9 &  53   & $1.1\times$ \\
  & ORT CPU$^\blacktriangle$        & FP32 & 32.5 &  30   & $0.6\times$ \\
  & ORT CPU$^{\blacktriangle\lozenge}$ & FP32 & \textbf{13.4} & \textbf{75} & $\mathbf{1.5\times}$ \\
\midrule
\multirow{3}{*}{\shortstack[l]{Intel Core i7-11800H\\(8-core, 45\,W)}}
  & PyTorch Fused (CPU)$^\ast$              & FP32 & 25.14 & 39.9  & $1.0\times$ \\
  & PyTorch JIT Frozen (CPU)              & FP32 & 20.5 & 48.9  & $1.2\times$ \\
  & ORT CPU$^\blacktriangle$        & FP32 & 38.7 & 25.6  & $0.6\times$ \\
  & ORT CPU$^{\blacktriangle\lozenge}$ & FP32 & \textbf{22.2} & \textbf{44.6} & $\mathbf{1.1\times}$ \\
\midrule
\multirow{2}{*}{\shortstack[l]{Apple iPad Pro M4\\(${\sim}10$\,W)}}
  & CoreML ANE$^{\clubsuit}$        & FP32 & 5.6 & 180 & $1.0\times$ \\
  & CoreML ANE$^{\clubsuit}$        & FP16 & 2.8 & 360 & $2.0\times$ \\
  & CoreML ANE$^{\clubsuit\lozenge}$        & FP16 & \textbf{1.4} & \textbf{715} & $\mathbf{4.0\times}$ \\
\midrule
\multirow{4}{*}{\shortstack[l]{Apple iPhone 12\\(${\sim}5$\,W)}}
  & CoreML ANE$^{\clubsuit}$        & FP32 & 25 & 40 & $1.0\times$ \\
  & CoreML ANE$^{\clubsuit}$        & FP16 & 4.2 & 240 & $6.0\times$ \\
  & CoreML ANE$^{\clubsuit\lozenge}$        & FP16 & \textbf{2.7}  & \textbf{375} & $\mathbf{9.4\times}$ \\
\midrule
\multirow{2}{*}{\shortstack[l]{Xiaomi Poco X3 NFC\\(${\sim}5$\,W)}}
  & TFLite GPU        & FP32 & 96.1 & 10 & $1.0\times$ \\
  & TFLite GPU        & FP16 & \bf 62.5 & \bf 16 & $\mathbf{1.5\times}$ \\

\bottomrule
\end{tabular}%
}
\end{table}
