# Supplementary material for: ZipDepth: Bringing Lightweight Zero-Shot Monocular Depth Anywhere, on Any Device
Source: arXiv:2607.08771 source file (2026-07-09)
Supplement: Supplementary file 4 [file memory_resolution.tex]

\begin{table}[h]
\centering
\caption{\textbf{Peak memory across resolutions} (NVIDIA RTX 3090, PyTorch backend). \textit{Weights} are constant across resolutions; \textit{Activations} denotes peak intermediate-tensor memory during the forward pass; \textit{Peak} is total memory allocated (weights + activations). TensorRT and CoreML manage memory independently via their own runtimes and are not directly comparable to these figures.}
\label{tab:memory_resolution}
\setlength{\tabcolsep}{3pt}
\scriptsize
\resizebox{\linewidth}{!}{%
\begin{tabular}{@{}l r r r r r r r r r r r r@{}}
\toprule
\multirow{2}{*}{\textbf{Resolution}} & \multicolumn{3}{c}{\textbf{Eager FP32}} & \multicolumn{3}{c}{\textbf{Fused FP32}} & \multicolumn{3}{c}{\textbf{Eager FP16}} & \multicolumn{3}{c}{\textbf{Fused FP16}} \\
\cmidrule(lr){2-4} \cmidrule(lr){5-7} \cmidrule(lr){8-10} \cmidrule(lr){11-13}
 & \textbf{Wt.} & \textbf{Act.} & \textbf{Peak} & \textbf{Wt.} & \textbf{Act.} & \textbf{Peak} & \textbf{Wt.} & \textbf{Act.} & \textbf{Peak} & \textbf{Wt.} & \textbf{Act.} & \textbf{Peak} \\
\midrule
$384\!\times\!384$     & 25.9 & 80.1 & 106.0 & 23.4 & 80.9 & 104.3 & 12.9 & 66.5 & 79.4 & 11.7 & 65.8 & 77.5 \\
$768\!\times\!1024$    & 25.9 & 275.2 & 301.1 & 23.4 & 275.4 & 298.8 & 12.9 & 166.0 & 179.0 & 11.7 & 165.5 & 177.2 \\
$1024^2$                & 25.9 & 352.9 & 378.8 & 23.4 & 353.8 & 377.2 & 12.9 & 256.8 & 269.7 & 11.7 & 256.7 & 268.4 \\
$1080\!\times\!1920$   & 25.9 & 666.6 & 692.5 & 23.4 & 667.1 & 690.5 & 12.9 & 474.6 & 487.6 & 11.7 & 475.2 & 487.0 \\
$1440\!\times\!2560$   & 25.9 & 1153.8 & 1179.7 & 23.4 & 1154.5 & 1178.0 & 12.9 & 817.7 & 830.6 & 11.7 & 817.3 & 829.1 \\
$2160\!\times\!3840$   & 25.9 & 2550.9 & 2576.8 & 23.4 & 2552.2 & 2575.6 & 12.9 & 1791.3 & 1804.3 & 11.7 & 1790.2 & 1801.9 \\
\bottomrule
\end{tabular}
}
\end{table}
