# Supplementary material for: ZipDepth: Bringing Lightweight Zero-Shot Monocular Depth Anywhere, on Any Device
Source: arXiv:2607.08771 source file (2026-07-09)
Supplement: Supplementary file 5 [file resolution_highres.tex]

\begin{table}[h]
\centering
\caption{\textbf{High-resolution throughput.}
$\clubsuit$~CoreML ANE, NPU/mobile path.}
\label{tab:highres}
\setlength{\tabcolsep}{5pt}
\small
\resizebox{\linewidth}{!}{%
\begin{tabular}{@{}l r r r r r r r@{}}
\toprule
\textbf{Resolution} & \textbf{Mpx} & \textbf{GMACs} & \textbf{RTX 3090} & \textbf{RTX 3070} & \textbf{Orin NX (50\,W)} & \textbf{Orin NX (15\,W)} & \textbf{iPhone 12$^\clubsuit$} \\
\midrule
$768\!\times\!1024$    & 0.79 & 16.06 & 192 & 79 & 50 & 9 & 75 \\
$1024^2$               & 1.05 & 21.41 & 149 & 61 & 38 & 7 & 50 \\
$1080\!\times\!1920$   & 2.07 & 42.53 & 78 & 31 & 18 & 3 & 20 \\
$1440\!\times\!2560$   & 3.69 & 75.28 & 47 & 17 & 10 & 2 & 12 \\
$2160\!\times\!3840$   & 8.29 & 169.61 & 21 & 6 & 5 & 0.8 & OOM \\
\bottomrule
\end{tabular}
}
\end{table}
