# Supplementary material for: ZipDepth: Bringing Lightweight Zero-Shot Monocular Depth Anywhere, on Any Device
Source: arXiv:2607.08771 source file (2026-07-09)
Supplement: Supplementary file 6 [file resolution_throughput.tex]

\begin{table}[h!]
\centering
\caption{\textbf{Throughput vs.\ input resolution.} PyTorch Fused, FP32. $\clubsuit$ NPU/mobile path. Resolutions include common square and non-square aspect ratios.}
\label{tab:resolution}
\setlength{\tabcolsep}{3.pt}
\small
\resizebox{\linewidth}{!}{%
\begin{tabular}{@{}l rrrrrrr@{}}
\toprule
\multirow{2}{*}{\textbf{Device}}
  & \multicolumn{7}{c}{\textbf{Input Resolution (FPS)}} \\
\cmidrule(l){2-8}
  & $256^2$ & $384^2$ & $384\!\times\!512$ & $512^2$ & $384\!\times\!672$ & $512\!\times\!768$ & $768\!\times\!1024$ \\
\midrule
RTX 3090 - GPU
  & 401 & 389 & 380 & 365 & 346 & 302 & 192 \\
RTX 3070 - GPU
  & 476 & 368 & 298 & 222 & 219 & 156 & 79\\
Orin NX - GPU (50\,W)
  & 141 & 118 & 116 & 108 & 110 & 94 & 50\\
Orin NX - GPU (15\,W)
  & 56 & 34 & 30 & 24 & 24 & 17 & 9\\
Intel i7-11800H - CPU
  & 72 & 41 & 27 & 20 & 22 & 15 & 7 \\
  \hline
  iPhone 12 A14
  & 44 & 40 & 37 & 30 & 28 & 20 & 10 \\
  iPhone 12 A14 (FP16)
  & 490 & 240 & 195 & 150 & 145 & 95 & 43 \\
iPhone 12 A14 (FP16)$^\clubsuit$
  & 675 & 375 & 315 & 245 & 235 & 160 & 75 \\
\bottomrule
\end{tabular}
}
\end{table}
